# Supplementary material for: Submodular Matroid Secretary Problem with Shortlists
Source: arXiv:2001.00894 source file (2020-01-03)
Supplement: Supplementary file 1 [file appendix.tex]

\subsection{Some useful properties of $(\alpha,  \beta)$  windows}
\label{app:windows}
Lemma \ref{lem:indep} is a corollary of the following lemma.
\begin{lemma}\label{eqprob}
For each $y\in [k\beta]^n$, $Pr\{Y=y\}=(\frac{1}{k\beta})^n$.
\end{lemma}
\begin{proof}
Consider pair $(\pi, \psi)$, where $\pi:I\to [n]$  defines the random order on $I$. 
Throw $n$ balls uniformly into $k\beta$ bins. Let $\psi_j$ be the  bin that $j$-th ball goes into. % and $X_i$ be the number of balls in the $i$-th bin.
Note that $\psi$ and $\pi$ are independent. Now consider
%For a given $y\in  [k\beta]^I$, 
\[
(\frac{1}{k\beta} s_1 + \cdots + \frac{1}{k\beta} s_{k\beta})^n = 
\left(\frac{1}{k\beta}\right)^n \sum_{t_1,\cdots, t_{k\beta}} Q_{t_1,\cdots, t_{k\beta}}  {s_1}^{t_1} \cdots  {s_{k\beta}}^{t_{k\beta}}\ .
\]
For a given $y\in  [k\beta]^I$,  suppose $t_i$ is the number of elements in slot $s_i$.
Then from above expansion the probability that $\psi$ divides input into slots of size $t_1,\cdots, t_{k\beta}$ is
\[
\left(\frac{1}{k\beta}\right)^n Q_{t_1,\cdots, t_{k\beta}}  =  \left(\frac{1}{k\beta}\right)^n {n \choose t_1, t_2, \cdots, t_{k\beta}}\ .
\]
Now for such a $\psi$, the probability that permutations $\pi$ satisfy $Y=y$ is 
\[
\frac{t_1! \cdots t_{k\beta}! }{n!}\ .
\]
Thus the probability that $Y=y$ is 
\[
\left(\frac{1}{k\beta}\right)^n {n \choose t_1, t_2, \cdots, t_{k\beta}} \frac{t_1! \cdots t_{k\beta}! }{n!} = \left(\frac{1}{k\beta}\right)^n\ .
\]

\end{proof}

%=========================================
\subsection{m-submodular functions}
\label{app:msubm}
\begin{definition}
We call a function $f:2^{A}\rightarrow \mathbb{R}, $ m-submodular if it is submodular and there exists a submodular function $F$ such that:
%\begin{itemize}
%\item 
%\mcomment{switch $f$ and $F$}
\[ 
f(S)= \max_{T\subseteq S, |T|\le m} F(T)\ .
\]
\end{definition}
%\end{itemize}
Note that  maximum node weighted bipartite matching and  maximum edge weighted bipartite matching defined on $G=(X\times Y)$ with $|Y|=m$ are m-submodular. 
(the assignments will be done at the end of algorithm after all the selections are made )

\begin{remark}
$f(S)=\max_{a\in S} a$ is a $1$-submodular function.
\end{remark}

Now consider the following simple greedy algorithm:

\begin{algorithm*}[ht]
  \caption{~\bf{Select-If-it-Improves}($f,I , u$)}
  \label{alg:SIII} 
\begin{algorithmic}[1]
\State $R\leftarrow \emptyset$
\For {i=0 to n}
\If {$f(R\cup \{a_i\}) > f(R) $} 
%and $|R\setminus \{a_1,\cdots, a_u\}|<L$}
\State $R\leftarrow R\cup \{a_i\}$
\EndIf
\EndFor
\State return $S\leftarrow R\setminus \{a_1,\cdots, a_u\}$
\end{algorithmic}
\end{algorithm*}

\scomment{the remark below is incorrect. We have changed Algorithm \ref{alg:SIIImax} to start at $u$, and also end once the shortlist is of size $L$.}

%\begin{remark}
%Algorithm~\ref{alg:SIIImax} is special case of Algorithm~\ref{alg:SIII} for  $F(S)=\max_{a\in S} a$.
%\end{remark}

\scomment{please use "theorem" very sparingly. Theorem should be used only for the main results of the paper. We should not have any theorems beyond the 4 results in "Our results" section. I have changed your "theorems" to "lemma"}
\begin{lemma}
Suppose $R$ is the set of elements selected in the above algorithm on the input $I=\{a_1,\cdots, a_n\}$ then $f(R) = f(I)$.
\end{lemma}
\begin{proof}
%Suppose $F(I)=f(T)$,  where $|T|=m$. The above algorithm never miss  any element of $T$.
%Since $F$ is submodular if the marginal increae
Suppose $R_i$ is the subset selected at iteration $i$. Since $f$ is submodular, if $f(R_i\cup \{a_i\}) \le f(R_i)$ 
then $f(R\cup\{a_i\}) \le f(R)$. Therefore every $e\in I\setminus R$ has marginal value 0 with respect to $R$, i.e., $f(R)=f(I)$.
\end{proof}

%Now let's define $S':=S\setminus \{a_1,\cdots, a_u\}$.

\begin{lemma}
$E[|S|] = m\ln(n/u)$.
\end{lemma}
\begin{proof}
Suppose $f(R_i) = F(T)$, where $|T|=m$. If $a_i \notin T$ then it is not selected. 
Because if $a_i\notin T$ and is selected then it should have positive $f$ marginal value, which means $f(R_i) = f(R_{i-1} \cup \{a_i\} ) > f(R_{i-1}) =  F(T) $, it is a contradiction. 
Thus only elements in $T$ will be selected at position $i$.  

If you consider all permutations of $R_i$, an element will be selected at position $i$ if it is subset of $T$, the probability is $|T|/i= m/i$. Therefore the total expected number of selections $\mathbb{E}[|R|]$, will be at most $\sum_{i=1}^{n} \frac{m}{i}  = m \ln n $. Similarly 
$\mathbb{E}[|S|] \le \sum_{i=u}^{n} \frac{m}{i}=m\ln(n/u)$.
%The expected number of elements selected at position $\ell$ is at most $\frac{m}{\ell}$. 
\end{proof}

\toRemove{
\begin{lemma}
$E[|S|] = m\log n$
\end{lemma}
\begin{proof}
Suppose $f(S_i) = F(T)$, where $|T|=m$. If $a_i \notin T$ then it is not selected. 
Because if $a_i\notin T$ and is selected then it should have positive $f$ marginal value, which means $f(S_i) = f(S_{i-1} \cup \{a_i\} ) > f(S_{i-1}) =  F(T) $, it is a contradiction. 
Thus only elements in $T$ will be selected at position $i$.  

If you consider all permutations of $S_i$, an element will be selected at position $i$ if it is subset of $T$, the probability is $|T|/i= m/i$. Therefore the total expected number of selections will be at most $\sum_{i=1}^{n} \frac{m}{i}  = m \ln n $
%The expected number of elements selected at position $\ell$ is at most $\frac{m}{\ell}$. 
\end{proof}
}

In the rest we will make the following assumption:\\
\textbf{Assumption. } %There is a unique $m$-tuple $OPT$ with maximum $f(OPT)$ in the input. 
There is a unique optimal solution OPT.

%\msub

\begin{lemma} \label{hprob}
Algorithm~\ref{alg:SIII}, with parameter $u=n\epsilon$,  selects a set $S$ with 
$$|S|<m\ln (1/\epsilon)+\ln(1/\delta)+\sqrt{\ln^2{1/\delta}+2m\ln(1/\delta)\ln(1/\epsilon)}$$ 
and $E[f(S)]=(1-\epsilon-\delta)OPT$.
\end{lemma}
\begin{proof}
We use Freedman's inequality.
 If $\{a_1,\cdots, a_i\}$ has a unique maximum subset of size $m$, define $Y_i$ to be a random variable indicating whether the algorithm has selected $a_i$  or not, where $Y_i=1-\frac{m}{i}$ if $a_i$ is selected and $Y_i=-\frac{m}{i}$ otherwise. 
 If it has not unique solution define $Y_i=0$. ($a_i$ will not be selected)
 Also define $\mathcal{f}_i=\{Y_{n},Y_{n-1}, \cdots, Y_{n-i+1}\}$.

Let $X_i=\sum_{j=n-i+1}^{n} Y_j$,
then $\{X_i\}$ is a martingle, 
because $E[X_{i+1}|\mathcal{f}_{i}] = X_i+E[Y_{n-i}|\mathcal{f}_i]$.
 If $\{a_1,\cdots, a_i\}$ has a unique maximum subset of size $m$, $E[Y_{n-i}|\mathcal{f}_i]=(m/i)(1-m/i)+(1-m/i)(-m/i)=0$,
 otherwise $E[Y_{n-i}|\mathcal{f}_i]=0$. So in both cases $E[X_{i+1}|\mathcal{f}_{i}] =X_i$.
%X_i+E[Y_{n-i}]=X_i$. Also $|X_{i+1}-X_i| < 1$.
%frac{m}{i} (1-\frac{m}{i}) +(1-\frac{m}{i})\frac{m}{i} 
As in the Freedman's inequality, let $L=\sum_{i=n\epsilon}^{n} Var(Y_i| f_{i-1})$. 
\begin{align*}
L  =  \sum_{i=n\epsilon}^{n} \frac{m}{i}  (1-\frac{m}{i})^2 + (1-\frac{m}{i}) (\frac{m}{i})^2 
< \sum_{i=n\epsilon}^{n} \frac{m}{i} =m\ln (1/\epsilon) \ .
\end{align*}
Therefore,
\[
Pr(X_{n-n\epsilon}\ge \alpha \text{ and }  L\le m\ln (1/\epsilon) ) \le exp(-\frac{\alpha^2}{2m\ln (1/\epsilon)+ 2\alpha })   < \delta \ .
\]
Thus we get $\alpha > \ln(1/\delta)+\sqrt{\ln^2{1/\delta}+2m\ln(1/\delta)\ln(1/\epsilon)}$.
%Thus we get $\alpha > \ln(1/\epsilon)(1+\sqrt{1+2m})$. 
Also $|S| = X_{n-n\epsilon} + m\ln(1/\epsilon)$. Therefore 
\[
Pr(|S| \ge  m\ln (1/\epsilon)+\ln(1/\delta)+\sqrt{\ln^2{1/\delta}+2m\ln(1/\delta)\ln(1/\epsilon)}  )  \le \delta\ .
\]
So with probability $(1-\delta)$, $|S| \le m\ln (1/\epsilon)+\ln(1/\delta)+\sqrt{\ln^2{1/\delta}+2m\ln(1/\delta)\ln(1/\epsilon)} $.  %\frac{m\ln c}{\sqrt{\epsilon}} + m\ln c $ .
%Suppose $OPT$ is the optimal solution, i.e $|OPT|=m$ and  $f(OPT)$ is maximum in subsets of $I$.
Since $F$ is submodular, $E[F(OPT\cap \{a_{n\epsilon},\cdots, a_n \} )] = (1-\epsilon)OPT$.
Therefore $E[f(S)] \ge (1-\epsilon)OPT-\delta OPT$. 
%By setting $1/c=\epsilon$, $|S|=m\ln (1/\epsilon)+ \sqrt{2m \log (1/\epsilon)} $ and $E[F(S)]=(1-2\epsilon)OPT$.
\end{proof}
\scomment{Considering that Remark 1 is incorrect,  proof of Proposition \ref{maxanalysis} does not directly follow from above. We need to explicitly add the proof of Proposition \ref{maxanalysis}. Or else you need modify Algorithm 3 so that Algorithm~\ref{alg:SIIImax} is a special case.}

%Note that a special case of $m$-submodular functions is $F(S) = \max_{a\in S} a$. Following the above lemma the proof of 
%\maxanalysis*

%\paragraph{Proof of Proposition \ref{opttheorem}.}  

\maxanalysis*
\begin{proof}
Set $u=n\delta/2$ and $\epsilon=\delta/2$, and $f(T):=\max_{a\in T} a$.
 The set $S$ returned by the Algorithm~\ref{alg:SIII} is the same as the set $A$ selected by Algorithm~\ref{alg:SIIImax},  when $|S|<L$.
From lemma~\ref{hprob} with probability $(1-\delta)$, $|S|<(3+\sqrt{2})\ln(2/\delta)<L$. 
Also $f(S)=A^*$.
Therefore w.p. $(1-\delta)$ Algorithm~\ref{alg:SIIImax} returns $A^*$.
\end{proof}

\scomment{What is the purpose of the results below? Are you trying to prove some lower bound? I am removing it.}
\toRemove{
\begin{lemma}
Any online algorithm needs to select at least $\frac{1}{2}\log(1/\epsilon)-\frac{1}{2}$ elements, in expectation, to select the maximum element  with probability at least $(1-\epsilon)$ in a random permutation. (we assume $n> 1/\epsilon$)
\end{lemma}
\begin{proof}
Let $I_i=\{a_1,\cdots, a_{n/2^{i-1}}\}$, $T_i=\{a_{n/2^i+1}, \cdots, a_{n/2^{i-1}}\}$, and $R_i=I_1\setminus I_i$, for $i=1, \cdots, \log(1/\epsilon)$. Suppose $M_i$ is the maximum element in $I_i$. Let $S$  be the set of selected elements by algorithm at the end of execution.
Suppose $\epsilon_i= E[M_i\notin S| M_i\in T_i]$,
then $E[|S\cap T_i|] \ge \frac{1}{2} (1-\epsilon_i)$.
Therefore $E[|S|] \ge \sum_{i=1}^{\log(1/\epsilon)} \frac{1}{2} (1-\epsilon_i) $. Also w.p. $\frac{1}{2^{i}}$, $M_1 \in T_i$, 
thus $\sum_{i=1}^{\log(1/\epsilon)} \frac{1}{2^{i}} \epsilon_i  \le \epsilon$. 
(Note that we use the fact $ E[M_i\notin S| M_i\in T_i \text{ and }  M_i=M_1] \le \epsilon_i$, i.e, if algorithm selects one element it will select 
it even if we increase its value and keep the rest untouched) 
Now $E[|S|]$ is minimized under above constraint if $\frac{1}{2^{\log(1/\epsilon)}}\epsilon_{\log(1/\epsilon)} = \epsilon$ and the rest are zero.
Hence $E[|S|] \ge \frac{1}{2}\log(1/\epsilon)-\frac{1}{2}$.
\end{proof}
\begin{prop}
For a m-submodular function $F$, any online algorithm needs to select at least $\frac{m}{2}\log(m/\epsilon)-\frac{m}{2}$ elements, in expectation, to select a set $S$, with $|S|\le m$  such that  $E[F(S)] \ge (1-\epsilon)OPT$, in a random permutation. 
\end{prop}
\begin{proof}
Apply previous theorem on m separate 1 to n matching.
\end{proof}
}
\toRemove{
\subsection{A special family of monotone submodular functions}
%Submodular maximization 
We find some assumption for sumbmodular functions under which the Kleinberg's algorithm gives asymptotic optimal solution.
%The condition is more general than the assumption regarding the curvature of submodular functions.
%We will define the precise condition below:
We consider special submodular functions that are defined on real value elements. In other words, submodular function $f$ defined on a ground set $X\subseteq \mathbb{R}$. i.e., $f:2^{X} \rightarrow \mathbb{R}$. 
With some reasonable assumptions 
%such as $F$ being commutative and associative 
we can represent $f$ in a simpler way.
%First let's elaborate on what we mean by commutative and assosiative. 
%A function $g:\mathbb{R}^n \rightarrow \mathbb{R}$ is commutative if $g(x_1,\cdots, x_n) = g(x_{\sigma_1}, \cdots, x_{\sigma_n})$ for every permutation $\sigma \in \Pi_n$. 
%We can represent $f$ in a different way.  
Let's define $f(x_1,\cdots, x_k) = f(\{x_1, \cdots, x_k\})$, where $k$ is the number of items we are allowed to select from the input.
%the original representaton $f(0,1,0,0,0,1,1,0) \in \mathbb{R}$.
The value of $k$ elements $a_1, \cdots, a_k$ selected from the ground set is $f(\{a_1, \cdots, a_k\})$.
We can also represent it by symmetric function $f(a_1,\cdots, a_k)$. 
%since it is commutative we can say this value is invariant under any permutation. 
%So basically we can say the value if any selection of $k$ elements $a_1, \cdots, a_k$ from the ground set can be defined by the symmetric function $F(a_1, \cdots, a_k )$. 

Now we focus on properties of $f:\mathbb{R}^k \rightarrow \mathbb{R}$. ( Note the domain of  $f:2^X \rightarrow \mathbb{R}$)
%What does submodularity of $f$ imply for $F$?
%Submodular property for $f$: $f(S \cup \{a_i\} ) \ge f(S'\cup \{a_i\}) $ for $S'\subseteq S$.
%which is equivalent to the following: $F(a_1,\cdots, a_k)$ vs $F(a_1, \cdots, a_k + \alpha )$, where $\alpha >0$. 
%We claim that under commutative assumption $F(a_1,\cdots,a_i+\alpha,\cdots, a_k)  \ge  F(a_1, \cdots, a_i, \cdots, a_k  )$.
By making the following assumptions about $f$, we will show Kleinberg's algorithm asymptotically approaches optimal solution.
%The first one implies the second one and the second one is more general assumption but the first one is related to the notion of curveture of a submodular fucntion.

\begin{enumerate}
\item $f$ is a monotone submodular function and $f(a_1,\cdots, a_i+\alpha,\cdots, a_k)  \ge  f(a_1, \cdots, a_i, \cdots, a_k  )$, for $\alpha >0$ and $1\le i \le k$.

\end{enumerate}

%\begin{claim}
%If $f(\{x\}) \rightarrow \infty$ as $x\rightarrow \infty$, then $F(a_1,\cdots, a_i+\alpha,\cdots, a_k)  \ge  F(a_1, \cdots, a_i, \cdots, a_k  )$, for $\alpha >0$ and $1\le i \le k$.
%\end{claim}
%\begin{proof}
%Suppose it is not. Thus there exists $i$ and $\alpha>0$ such that $F(a_1,\cdots, a_i+\alpha,\cdots, a_k)  <  F(a_1, \cdots, a_i, \cdots, a_k  )$ 
%\end{proof}
%A more general claim is that there is an optimal offline solution that consists of the top $k$ largest elements.

An immediate consequence of this assumption is that the optimal offline solution is the set of $k$ largest elements in the input (not necessarily unique).
%Suppose $X=\{a_1 > a_2 > \cdots > a_n\}$.  Then the optimal offline solution is $f(\{a_1,\cdots, a_k\})$ (not necessarily unique).
%i.e., $f(a_1, \cdots, a_k) \ge f(a_{j_1}, \cdots, a_{j_k})$.
Now we claim that the Kleinberg algorithm works under this assumption which means that the competitive ratio of the algortihm assymptotically approaches to 1.

%Before proving the theorem we  just mention how the assumption above is related to curveture of a submodular function.
%The \textit{total curveture} of $f$ is defined as $c=1-\min_{S,j\notin S} \frac{f_S(j)}{f_{\emptyset}(j)}$. Note that $c\in [0,1]$.
%The assumption above is equivalent to $c<1$.

\subsubsection{Analysis of Kleinberg's Algorithm }

%Just a reminder of the main property that we assume during this section: 
Suppose $X=\{x_1 \ge x_2 \ge \cdots \ge x_n\}$.  We assume the optimal offline solution is $\{x_1,\cdots, x_k\}$ (not necessarily unique).
i.e., $f(\{x_1, \cdots, x_k\}) \ge f(\{x_{j_1}, \cdots, x_{j_k}\})$.
The sketch of our approach is to show that the Kleinberg algorithm in fact selects $(1-5/\sqrt{k}).k$ many elements from top $k$ elements of input, i.e., $x_1, x_2, \cdots, x_k$. 
Suppose we have two subsets $S,U\subseteq X$. We say $S\ge U$ if $S=\{p_1\ge p_2 \ge \cdots \ge p_r\}$ and $U=\{q_1 \ge \cdots \ge q_r\}$, and $p_1 \ge q_1, \cdots, p_r>q_r $. Note that because of property (1), $f(S)>f(U)$.
%Then we argue that a sorted $k$-tuples is larger than some other $k$-tuple, it will be selected by the algorithm with higher probability.  
We denote by $P_S$ the probability that the algorithm selects all the elements of $S$ from the input. For $S,U \subseteq X$ and $S \ge U$  we show that $P_S \ge P_U$.
Therefore the expected value of items selected by the algorithm is at least as much as when we select $(1-5/\sqrt{k}).k$  many items uniformly at random, in which case because of monotonicity and submodularity we can say that  its expected value is at least $(1-5/\sqrt{k}).f(x_1,\cdots, x_k)$.
%Remember for the case $f$ is sum, $OPT$ consists of the top $k$ elements of input.

Now we remind the Kleinberg algorithm. 
Suppose the input sequence is $a_1, \cdots, a_n$, and we want to irrevocably select $k$ elements in an online manner.
The algorithm recursively divides the input into two halves:
It draws a random variable $m$ from binomial distribution $m=B(n, 1/2)$. 
Recursively select $\ell =\lfloor k/2 \rfloor$ elements from $a_1, \cdots, a_{m}$. 
Suppose $y_1> y_2 > \cdots > y_m$ are the elements in the first half.
After observing $a_m$, select every element which exceeds $y_{\ell}$, until we have selected $k$ items or have seen all elements of $S$. 

%One idea in the analysis is that they define the modified value of an element to be 0 if the elements is not among the top $k$ elements of the input and its value if it is one of the top $k$ elements. 
Let $T\subseteq S$ denote the $k$ largest elements of $S$. In the analysis they set to 0 every element which is not among the top $k$ elements, and call it the modified value of that element, ie.,
modified value of an element $x \in S$ is equal to its value if $x \in T$ and zero otherwise; 
%the modified value of a set is the sum of the modified values of its elements.

\begin{theorem}
Let $S$ be any set of $n$ non-negative real numbers. Let $T$ be the $k$ largest elements of $S$, and $OPT=f(T)$.
The expected number of elements of $T$ selected by the algorithm is at least $(1 -5/\sqrt{k})k$.
\end{theorem}
\begin{proof}
%Let $T\subseteq S$ denote the $k$ largest elements of $S$. Define the modified value of an element $x \in S$ to be equal to its value if $x \in T$ and zero otherwise; the modified value of a set is the sum of the modified values of its elements. 
%We will prove that the expected number of elements of $T$ selected by the algorithm is at least $(1 - 5/\sqrt{k})k$. 
The proof is by induction on $k$. % paralleling the recursive structure of the algorithm.
Let $y_1 >y_2 >\cdots >y_m$ be the first $m$ samples, and let $z_1 > z_2 > . . . > z_{n-m}$ be the remaining samples; denote these sets by $Y$ and $Z$ respectively. 
%Since $m$ has distribution $B(n,1/2)$, it follows that $Y$ is a sample from the uniform distribution on all $2^n$ subsets of $S$. In particular, $Y \cap T$ is a uniform random subset of $T$. This has the following consequences. 
%First, the random variable $|Y \cap T |$ has the distribution $B(k,1/2)$. 
%Second, 
Conditional on the event $|Y \cap T | = r$, 
%the expected number of elements of $OPT$ in $Y$ is $(r/k)k$ (because of monotonicity and submodularity of $f$ and random sampling). 
%Also, the expected modified value of the top $\ell = k/2$ elements of $Y$ is bounded below by
the expected number of the top $\ell = k/2$ elements of $Y\cap T$ is bounded below by

\[
\sum_{r=1}^{k} Pr(|Y \cap T|=r) . (\min(r,l)/k) k \ge (1-\frac{1}{2\sqrt{k}}) \frac{k}{2}.
\]

Thus the expected number of elements selected from $Y\cap T$ is
at least $(1-5/ \sqrt{k/2})·(1-1/2\sqrt{k}).(k/2)$, by the induction hypothesis.
%\end{proof}

%Now we turn to estimating the modified value of the elements selected from $Z$. 
Similar to Kleinberg define the random variable $q$ which counts the number of elements of $Z$ exceeding $y_{\ell}$. Let $q_i$ be the number of elements of $Z$ whose value lies between $y_i$ and $y_{i-1}$. The $q_i$ are stochastically dominated by i.i.d. geometrically distributed random variables each having mean 1 and variance 2.
Thus their sum $q =  \sum_{i=1}^{\ell} q_i$ satisfies $E[|q-\ell|] \le \sqrt{k}$.
%Let $r=|q-\ell|$. An easy argument shows that the expected number of elements of $Z\cap T$ selected by the algorithm, conditional on $r$, is at least $(1/2 - r/k) k = \ell - r= \ell- |q-\ell| = q$.
Let $r=|q-\ell|$. The expected number of elements algorithm selects from $Z\cap T$ is at least $ \ell-r$ (if $y_{\ell} \in T$ the argument is similar to Kleinberg if $y_{\ell} \notin T$ Then all the elements of $Z \cap T$ will be selected  ). 
Removing the conditioning on $r$ and recalling that $E(r) \le \sqrt{k}$, the algorithm selects a subset of $Z$ with expected size $\ell-\sqrt{k}$. Combining this with the above paragraph will show that the expected number of elements selected from $Y\cup Z$ is $(1-5/\sqrt{k})k$.

\end{proof}

If the algorithm could  select  these subsets  uniformly at random then because of submodularity the  expected value of function $f$ that the algorithm selects from $T$ will  be $(1-5/\sqrt{k})OPT$.
%$Z\cap T$ would be $(\ell-\sqrt{k}).OPT/k = (1/2-\sqrt{1/k})OPT$. %(conditions of this property? montonicity)
Next lemma will prove the expected value of selected elements by the algorithm is at least as much as uniform case.

\begin{lemma}
%For $S,U \subseteq X$ and $S \ge U$  we show that $P_S \ge P_U$.
If $T=\{a_1,a_2, \cdots, a_k\}$ and $a_1>a_2> \cdots > a_k$, the probability that the algorithm selects $a_i$ is larger than the probability it selects $a_j$ for $i<j$.
\end{lemma}
\begin{proof}
%Now we claim that if $b_1\ge b_2 \ge \cdots \ge b_{\ell}$ and $c_1 \ge c_2 \ge \cdots \ge c_{\ell}$ are two subsets of $Z$, and $b_i \ge c_i$ for $1 \le i \le \ell$. Then the probability that the algorithm selects $b_i$s is greater than the probability that the algorithm selects $c_i$s. 
%The reason is the following:  
Let's fix the set $Y$ and $Z$ but not the ordering of elements in $Z$.
the algorithm selects all the elements of $Z$ greater than $y_{\ell}$ until it selects $\ell$ elements.
So among all different possible permutations for $Z$, the algorithm will select the first $\ell$ elements of $Z$ greater than $y_{\ell}$.
If the total number of these elements, $t$, is less than or equal to $\ell$ then regardless of permutation of elements in $Z$ we select the same subset of $Z$ (the $t$  largest elements of $Z$).  

We should see what elements of $T\cap Z$ will be missed by the algorithm, and show that the smaller an element is the larger the probability of missing that item is. Suppose $a\in T\cap Z$, it will be missed by the algorithm if either $a\le y_{\ell} $ or $a \ge y_{\ell}$ but there are $\ell$ elements larger than $y_{\ell}$ appearing before $a$ (after selecting $\ell$ elements the rest are truncated).

If $a,b\in Z$  and $a>b$ the probability that we miss $a$ for the first reason is less than the probability that we miss $b$ for the first reason.
Also if both $a$ and $b$ pass the condition of second case, i.e., $a> y_{\ell}$ and $b> y_{\ell}$ then they are both equally likely to be missed by algorithm (only depend on their position in the the input). 
So $b$ is more likely to be missed by the algorithm.  

If $a,b \in Y$ then by induction you can show the probability that $a$ is selected is larger than the probability that $b$ is selected.

Now consider the case that one of $a$ or $b$ is in $Y$ and the other is in $Z$. The probability that $a\in Y, b\in Z$ is the same as the probability $b\in Y, a\in Z$. 
By switching the place of $a$ and $b$ and fixing the rest, the probability that $a$ is selected in $Y$ is larger than the probability $b$ is selected because if $b$ is larger than threshold, $a$ is too. If $a$ is missed for truncation, $b$ will also be truncated if we replace it in the same place as $a$ is in $Y$.
For the $Z$ part, if $a\in Y, b\in Z$, the threshold $y_{\ell}$ is larger than or equal the case $b\in Y, a\in Z$. Thus if $b$  is not missed in $Z$ with the larger threshold, $a$ which is larger than $b$ will not be missed with the smaller threshold. 
%Similarly, the probability that $a$ is selected in $Z$ is also larger than the probability that $b$ is selected.

Hence the probability that the algorithm misses $a_i$ is less than or equal the probability that it misses $a_{i+1}$.
%So if $h_1 > h_2> \cdots > h_{k'}$ are the elements of $T\cap Z$,  the probability that the algorithm misses $h_i$ is less than or equal the probability that it misses $h_{i+1}$.

\end{proof}

\begin{lemma}
Assuming the expected number of elements that the algorithm selects is $(1-5/\sqrt{k}).k$, and $p_1>p_2>\cdots> p_k$ are respectively the probability that  each element of $T=\{a_1>\cdots>a_k\}$ is selected, then $E[f(S)]>(1-5/\sqrt{k})OPT$, where $S$ is the subset of $T$ selected by the algorithm.
\end{lemma}
\begin{proof}
%Suppose $\sum_{i=1}^k p_i=q$
First by induction on $k$, we prove that the probability distribution $\Pi$ over subsets of $T=\{a_1,\cdots, a_k\}$ that minimizes $E_{\Pi, S\in T} f(S)$, is the following distribution: $\Pi(\{a_1,\cdots, a_t\})=(p_t-p_{t+1})$,  $1 \le t\le k$. Suppose $p_{k+1} = 0$, and $P(\emptyset) = 1-p_1$.

For $k=1$,  $\Pi(\{a_1\})=p_1$ and $\Pi(\emptyset)=1-p_1$. Hence $E_{\Pi}[f(S)]=p_1f(\{a_1\})=p_1.OPT$, which is the only option.

%Now suppose for $k-1$, the above distribution is a minimizer.  We want to show that the 
Now we want to show that the above distribution is a minimizer for $T$. By projecting $\Pi$ to subsets of $T'=\{a_1,\cdots, a_{k-1}\}$, say $\Pi'$ , we have $\Pi'(S)= \Pi(S)+\Pi(S\cup\{a_k\})$, $\forall S\subseteq T'$. The marginal probabilities of elements in $T'$ are $p_1>\cdots > p_{k-1}$. By induction the $\Pi'$ is the minimizer of $E_{\Pi', S\in T'}[f(S)]$. Now we show $\Pi$ is minimizer of for $T$. Consider a different distribution $\Theta$. Suppose $\Theta'$ is its projection to $T'$. 
\[
E_{\Theta, S \in T} f(S) = \sum_{S\subseteq T} \Theta(S) f(S)= \sum_{S\subseteq T'} (\Theta(S) f(S)+ \Theta(S\cup\{a_k\}) f(S\cup\{a_k\}) )  = 
\]
\[
E_{\Theta', S\in T'} f(S) +  \sum_{S\subseteq T'} \Theta(S\cup \{a_k\})  (f(S\cup\{a_k\}) - f(S)) 
\]
\[
\ge E_{\Pi', S\in T'} f(S) + p_k  (f(T) - f(T'))  = E_{\Pi, S\in T} f(S).
\]

Therefore  $\Pi$ is minimizer for $T$. (the last inequality is because of submodularity and induction hypothesis)

Now we lowerbound $E_{\Pi,  S\in T} f(S)$
\[
E_{\Pi,  S\in T} f(S) = \sum_{S\subseteq T} \Pi(S) f(S)  = \sum_{t=1}^{k} f(\{a_1,\cdots, a_t\}) (p_t-p_{t+1}) 
\]
\[
\ge \sum_{t=1}^{k} \frac{t}{k}OPT (p_{t} - p_{t+1})  = \frac{OPT}{k} \sum_{t=1}^{k} p_i 
\]

Thus The expected output of Kleinberg algorithm is at least $\frac{OPT}{k}(\sum_{i=1}^{k}) p_i = (1-5/\sqrt{k}) OPT$

%The marginal distribution that minimizes
%$E[f(S)]$ is $p_k.f(a_1,\cdots, a_k) + (p_{k-1}-p_k).f(a_1,\cdots, a_{k-1})+(p_3-p_2).f(a_1,\cdots,a_{k-2}) + \cdots +(p_1-p_2).f(a_1) $
%$\ge p_k.OPT+(p_{k-1}-p_k).\frac{k-1}{k}OPT+ \cdots + (p_1-p_2)\frac{1}{k} OPT  = \frac{OPT}{k} (p_1+\cdots+p_k)= \frac{OPT}{k} (1-5/\sqrt{k})k$.

\end{proof}
}
